# Supplementary material for: QuYBE -- An Algebraic Compiler for Quantum Circuit Compression
Source: arXiv:2212.06948 source file (2022-12-13)
Supplement: Supplementary file 1 [file appendix.tex]

%\appendix
\appendices
\section{Algebraic Condition for Reflection Symmetry}
\noindent \textbf{Theorem I~\cite{YBE_pra}} Given the time evolution operator that takes the following form,
\begin{align}
\mathcal{R}(\gamma,\delta) & =  
\begin{pmatrix}
   e^{i\delta}\cos(\gamma) & 0 & 0 & ie^{i\delta}\sin(\gamma) \\
   0 & e^{-i\delta}\cos{\gamma} & ie^{-i\delta}\sin{\gamma} & 0 \\
   0 & ie^{-i\delta}\sin{\gamma} & e^{-i\delta}\cos{\gamma} & 0 \\
   ie^{i\delta}\sin(\gamma) & 0 & 0 & e^{i\delta}\cos(\gamma)
   \end{pmatrix}, \label{propagator}
\end{align}
 the following YBE holds
\begin{align}
    &(\mathcal{R}(\gamma_1,\delta_1) \otimes \mathds{1})
    (\mathds{1} \otimes \mathcal{R}(\gamma_2,\delta_2))
    (\mathcal{R}(\gamma_3,\delta_3) \otimes \mathds{1})  \notag \\
    &~~~~=(\mathds{1} \otimes \mathcal{R}(\gamma_4,\delta_4))
    (\mathcal{R}(\gamma_5,\delta_5) \otimes \mathds{1})
    (\mathds{1} \otimes \mathcal{R}(\gamma_6,\delta_6)) \label{YBE2}
\end{align}
if and only if the following condition is satified
\begin{align}
&\left( \begin{array}{r} c_{\gamma_1-\gamma_3}s_{\delta_2} \\ c_{\gamma_1+\gamma_3}c_{\delta_2} \\ -s_{\gamma_1-\gamma_3}s_{\delta_2} \\ s_{\gamma_1+\gamma_3}c_{\delta_2} \end{array} \right)
\left( \begin{array}{r} c_{\delta_1-\delta_3}s_{\gamma_2} \\ c_{\delta_1+\delta_3}c_{\gamma_2} \\ -s_{\delta_1-\delta_3}s_{\gamma_2} \\ s_{\delta_1+\delta_3}c_{\gamma_2} \end{array} \right)^T  \notag \\
&~~~~~~~~~~~~~~~~~~= \left( \begin{array}{r} c_{\gamma_5}s_{\delta_4+\delta_6} \\ c_{\gamma_5}c_{\delta_4+\delta_6} \\ s_{\gamma_5}s_{\delta_4-\delta_6} \\ s_{\gamma_5}c_{\delta_4-\delta_6} \end{array} \right)
\left( \begin{array}{r} s_{\gamma_4+\gamma_6}c_{\delta_5} \\ c_{\gamma_4+\gamma_6}c_{\delta_5} \\ s_{\gamma_4-\gamma_6}s_{\delta_5} \\ c_{\gamma_4-\gamma_6}s_{\delta_5} \end{array} \right)^T, \label{L2R}
\end{align}
where $s_{p}$ and $c_{p}$ denote $\sin{(p/2)}$ and $\cos{(p/2)}$, respectively. \\
